# Supplementary material for: Quantum commitments and signatures without one-way functions
Source: arXiv:2112.06369 source file (2022-02-14)
Supplement: Supplementary file 1 [file appendix.tex]

{\color{red}\section{Appendix}}

\begin{definition}[Statistically distinguishable but computationally indistinguishable (SDCID) state generator]
A QPT algorithm $G$ is called statistically distinguishable but computationally indistinguishable (SDCID) state
generator if the followings are satisfied:
\begin{itemize}
\item
On input $b\in\bit$ and $1^\lambda$, $G$ applies a QPT unitary $U_b$ on $|0...0\rangle$
to generate $|\Psi_b\rangle_{AB}\equiv U_b|0...0\rangle$.
\item
$F(\rho_0,\rho_1)=\negl(\lambda)$,
where $\rho_b\equiv\mbox{Tr}_A(|\Psi_b\rangle\langle\Psi_b|_{AB})$.
\item
$\rho_0$ and $\rho_1$ are computationally indistinguishable with $\negl(\lambda)$ advantage.
\end{itemize}
\end{definition}

\begin{lemma}
$\mbox{Tr}(\rho_b^2)\le \negl(\lambda)$ for $b\in\bit$.
\end{lemma}

\begin{proof}
If the adversary generates $\rho_0$ and does the SWAP test between $\rho_0$ and the received state,
the computational indistinguishability requires
\begin{eqnarray*}
|\mbox{Tr}(\rho_0^2)-\mbox{Tr}(\rho_0\rho_1)|\le\negl(\lambda).
\end{eqnarray*}
Note that
\begin{eqnarray*}
\mbox{Tr}(\rho_0\rho_1)\le F(\rho_0,\rho_1)\le\negl(\lambda),
\end{eqnarray*}
and therefore $\mbox{Tr}(\rho_0^2)\le\negl(\lambda)$ has to be satisfied. 
\end{proof}

\begin{theorem}
SDCID state generators exist if and only if non-interactive quantum commitments with computational hiding
and statistical sum-binding exist.
\end{theorem}

\begin{theorem}
If 1-PRS generators for $m>cn$ with constant $c>1$ exist, SDCID state generators exist.
\end{theorem}

\begin{proof}
Let $\StateGen$ be a 1-PRS generator.  
Let us define a SDCID state generator $G$ as follows.
Its input is $1^n$ and $b\in\bit$.
When $b=0$, it generates 
$\frac{1}{\sqrt{2^n}}\sum_{k\in\bit^n}(|k\rangle\otimes|\eta_k\rangle)_A\otimes|\phi_k\rangle_B$
by coherently running $\StateGen$.
When $b=1$, it generates
$\frac{1}{\sqrt{2^m}}\sum_{r\in\bit^m}|r\rangle_A\otimes|r\rangle_B$.
Then $\rho_0=\frac{1}{2^n}\sum_k|\phi_k\rangle\langle\phi_k|$
and $\rho_1=\frac{I^{\otimes m}}{2^m}$.
Due to the security of 1-PRS, $\rho_0$ and $\rho_1$ are computationally indistinguishable
with advantage $\negl(n)$.
Also, when $m>cn$, $F(\rho_0,\rho_1)\le\negl(n)$.
\end{proof}

Open problem: the existence of SDCID means the existence of 1-PRS?

Assume that the adversary $\cA$ does a POVM measurement $\{\Pi_\sigma\}_{\sigma\in\bit^n}$.
Then,
\begin{eqnarray*}
\Pr[\cA'\to1|b'=1]
&=&
\int d\mu(\psi)
\sum_{\sigma\in\bit^n}
\Pr\Big[\sigma\leftarrow \cA(|\psi\rangle^{\otimes t})\Big]|\langle\phi_\sigma|\psi\rangle|^2\\
&=& 
\int d\mu(\psi) \sum_{\sigma\in\bit^n}\mbox{Tr}\Big[\Pi_\sigma
|\psi\rangle\langle\psi|^{\otimes t}\Big]
\mbox{Tr}\Big[|\phi_\sigma\rangle\langle\phi_\sigma|\times|\psi\rangle\langle\psi|\Big]\\
&=&
\int d\mu(\psi) \sum_{\sigma\in\bit^n}
\mbox{Tr}\Big[(\Pi_\sigma\otimes|\phi_\sigma\rangle\langle\phi_\sigma|) |\psi\rangle\langle\psi|^{\otimes t+1}\Big]\\
&=&
\sum_{\sigma\in\bit^n}
\mbox{Tr}\Big[(\Pi_\sigma\otimes|\phi_\sigma\rangle\langle\phi_\sigma|) 
\int d\mu(\psi) 
|\psi\rangle\langle\psi|^{\otimes t+1}\Big]\\
&=&
\sum_{\sigma\in\bit^n}
\mbox{Tr}\Big[(\Pi_\sigma\otimes|\phi_\sigma\rangle\langle\phi_\sigma|) \\
&&\times\frac{1}{(t+1)!}
{2^m+t\choose t+1}^{-1}
\sum_{\eta\in S_{t+1}}
\sum_{x_1,...,x_{t+1}\in{\mathcal X}}
|x_{\eta^{-1}(1)},...,x_{\eta^{-1}(t+1)}\rangle\langle x_1,...,x_{t+1}|
\Big]\\
&=&
\frac{1}{(t+1)!}
{2^m+t\choose t+1}^{-1}
\sum_{\sigma,\eta,x_1,...,x_{t+1}}
\langle x_1,...,x_t| \Pi_\sigma |x_{\eta^{-1}(1)},...,x_{\eta^{-1}(t)}\rangle
\langle x_{t+1}|\phi_\sigma\rangle\langle\phi_\sigma|x_{\eta^{-1}(t+1)}\rangle\\
&\le&
\frac{1}{(t+1)!}
{2^m+t\choose t+1}^{-1}
\sum_{\sigma,\eta,x_1,...,x_t}
\langle x_1,...,x_t| \Pi_\sigma |x_{\eta^{-1}(1)},...,x_{\eta^{-1}(t)}\rangle\\
&=&
\frac{1}{(t+1)!}
{2^m+t\choose t+1}^{-1}
\sum_{\eta,x_1,...,x_t}
\langle x_1,...,x_t|x_{\eta^{-1}(1)},...,x_{\eta^{-1}(t)}\rangle\\
&=&
\frac{1}{(t+1)!}
{2^m+t\choose t+1}^{-1}
\sum_{x_1,...,x_t}\\
&=&
\frac{1}{(t+1)!}
{2^m+t\choose t+1}^{-1}
2^{mt}\\
&\le&
\frac{1}{2^m}.
\end{eqnarray*}
Here, ${\mathcal X}$ is the $2^m$-dimensional Hilbert space, and each $x_i\in{\mathcal X}$
is a basis.
{\color{red}the seventh inequality does not work!}
